# Supplementary material for: Visualizing strongly focused 3D light fields in an atomic vapor
Source: arXiv:2506.01680 source file (2025-06-02)
Supplement: Supplementary file 1 [file BigDiagramSupplemental.pdf]

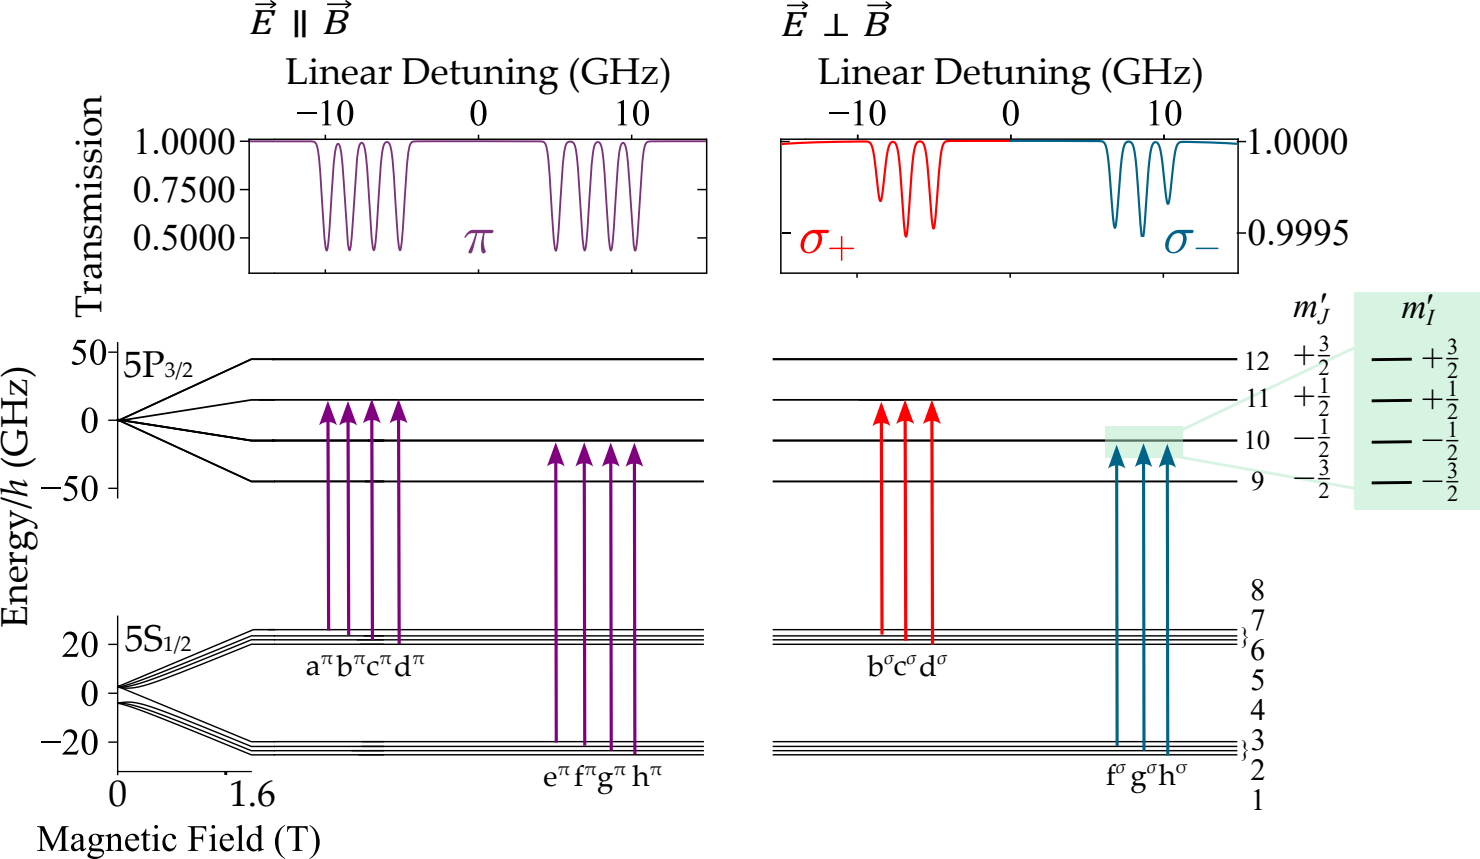

$|m_J, m_I\rangle$  state #:

8:  $1.0000 \left| +\frac{1}{2}, +\frac{3}{2} \right\rangle$

7:  $0.9979 \left| +\frac{1}{2}, +\frac{1}{2} \right\rangle + 0.0647 \left| -\frac{1}{2}, +\frac{3}{2} \right\rangle$

6:  $0.9968 \left| +\frac{1}{2}, -\frac{1}{2} \right\rangle + 0.0805 \left| -\frac{1}{2}, +\frac{1}{2} \right\rangle$

5:  $0.9971 \left| +\frac{1}{2}, -\frac{3}{2} \right\rangle + 0.0759 \left| -\frac{1}{2}, -\frac{1}{2} \right\rangle$

4:  $1.0000 \left| -\frac{1}{2}, -\frac{3}{2} \right\rangle$

3:  $0.9971 \left| -\frac{1}{2}, -\frac{1}{2} \right\rangle - 0.0759 \left| +\frac{1}{2}, -\frac{3}{2} \right\rangle$

2:  $0.9968 \left| -\frac{1}{2}, +\frac{1}{2} \right\rangle - 0.0805 \left| +\frac{1}{2}, -\frac{1}{2} \right\rangle$

1:  $0.9979 \left| -\frac{1}{2}, +\frac{3}{2} \right\rangle - 0.0647 \left| +\frac{1}{2}, +\frac{1}{2} \right\rangle$
